# Supplementary material for: Theory of Stochastic Drift
Source: arXiv:2406.14589 source file (2024-06-19)
Supplement: Supplementary file 1 [file additional_commands.tex]

%%%%%%%%%%%%%%%%%%%%%%%%
% Macros for the title %
%%%%%%%%%%%%%%%%%%%%%%%%

% The name of the authors.
\newcommand*{\printAuthor}{}
\newcommand*{\authorName}[1]{\renewcommand*{\printAuthor}{#1}}

% The name of the document.
\newcommand*{\printTitle}{}
\newcommand*{\titleName}[1]{\renewcommand*{\printTitle}{#1}}

% The name of the lecture.
\newcommand*{\printLecture}{}
\newcommand*{\lectureName}[1]{\renewcommand*{\printLecture}{#1}}

% The name of the lecture in short format.
\newcommand*{\printLectureShort}{}
\newcommand*{\lectureNameShort}[1]{\renewcommand*{\printLectureShort}{#1}}

% The name of the term.
\newcommand*{\printTerm}{}
\newcommand*{\termName}[1]{\renewcommand*{\printTerm}{#1}}

% The name of the term.
\newcommand*{\printHandInDate}{}
\newcommand*{\dateToHandIn}[1]{\renewcommand*{\printHandInDate}{Alle Aufgaben bis \textbf{#1}}}

\newcommand*{\printHandInDateQuiz}{}
\newcommand*{\dateToHandInQuiz}[1]{\renewcommand*{\printHandInDateQuiz}{Verständnisquiz (Moodle) bis \textbf{#1}}}

\newcommand*{\printHandInDatePrep}{}
\newcommand*{\dateToHandInPrep}[1]{\renewcommand*{\printHandInDatePrep}{Vorbereitungsaufgaben bis \textbf{#1}}}

\newcommand*{\printHandInDateRiddle}{}
\newcommand*{\dateToHandInRiddle}[1]{\renewcommand*{\printHandInDateRiddle}{Beweis-/ Knobelaufgaben bis \textbf{#1}}}

\newcommand*{\printHandInDateBonus}{}
\newcommand*{\dateToHandInBonus}[1]{\renewcommand*{\printHandInDateBonus}{Bonusaufgaben bis \textbf{#1}}}

% The name of the term.
\newcommand*{\printHandInNote}{}
\newcommand*{\handInLocation}[1]{\renewcommand*{\printHandInNote}{#1}}


%%%%%%%%%%
% Format %
%%%%%%%%%%

\newcommand*{\infobox}[1]
{%
    \begin{tabular}{!{\color{stroke1}\vrule width 2pt}p{\textwidth - 1.5 em}!{\color{gray!15}\vrule width 2pt}}%
        \rowcolor{gray!15}\vspace*{-5 pt}%
        #1%
        \vspace*{2.5 pt}%
    \end{tabular}%
    \bigskip%
}


%%%%%%%%%%%%%%%
% Other stuff %
%%%%%%%%%%%%%%%

% Indicator function
\newcommand*{\indicator}[1]{\mathOrText{\mathbf{1}{\{#1\}}}}

% Random process
\DeclareDocumentCommand{\randomProcess}{m o}
{%
    \mathOrText{X^{(#1)}\IfNoValueTF{#2}{}{_{#2}}}%
}

% Transformed process
\DeclareDocumentCommand{\transformedProcess}{o}
{%
    \mathOrText{Y\IfNoValueTF{#1}{}{_{#1}}}%
}

% Filtration
\DeclareDocumentCommand{\filtration}{o}
{%
    \mathOrText{\mathcal{F}\IfNoValueTF{#1}{}{_{#1}}}%
}

%\newcommand*{\N}{\mathOrText{\mathbf{N}}}
%\newcommand*{\R}{\mathOrText{\mathbf{R}}}
\newcommand*{\timePoint}{\mathOrText{t}}
\newcommand*{\stoppingTime}{\mathOrText{T}}
\newcommand*{\target}{\mathOrText{\alpha}}
\newcommand*{\drift}{\mathOrText{\delta}}
\newcommand*{\driftPositive}{\mathOrText{\delta^+}}
\newcommand*{\driftNegative}{\mathOrText{\delta^-}}
\newcommand*{\defeq}{\mathOrText{\coloneqq}}
\newcommand*{\eqdef}{\mathOrText{\eqqcolon}}
\newcommand*{\numberOfProcesses}{\mathOrText{k}}


% Vanja:
\renewcommand\thebonus{B\arabic{bonus}}
%\counterwithin*{equation}{exercise}

\renewcommand{\labelenumi}{(\alph{enumi})}
\renewcommand{\labelenumii}{(\roman{enumii})}

\newcommand*{\Oh}{\mathrm{O}}
\newcommand*{\Na}{\mathbb{N}}
\newcommand*{\Ra}{\mathbb{Q}}
\renewcommand*{\Re}{\mathbb{R}}
\DeclareMathOperator*{\argmax}{arg\,max}
\DeclareMathOperator*{\argmin}{arg\,min}
\newcommand*{\goed}{\textrm{göd}}
\newcommand*{\img}{\mathrm{img}}
\newcommand*{\myBigO}{\mathcal{O}}
% \newcommand*{\bigOmega}{\Omega}
% \newcommand*{\smallO}{\mathrm{o}}
% \newcommand*{\smallOmega}{\upomega}


\newcommand{\makeCompact}{%
\setlength{\itemsep}{1pt}%
\setlength{\parsep}{0pt}%
\setlength{\parskip}{0pt}}

\newcommand{\comment}[1]{\textcolor{blue}{[#1]}}
\newcommand{\ignore}[1]{}

% \newcommand{\set}[2]{\{ #1 \mid #2 \}}
\newcommand{\natnum}{\mathbb{N}}
\newcommand{\rationals}{\mathbb{Q}}
\newcommand{\integers}{\mathbb{Z}}
\newcommand{\realnum}{\mathbb{R}}
\newcommand{\Bij}{\mathcal{B}}

\newcommand{\isom}{\cong}

\newcommand{\FrakA}{\mathfrak{A}}
\newcommand{\converges}{\mathclose{\hbox{$\downarrow$}}}
\newcommand{\diverges}{\mathclose{\hbox{$\uparrow$}}}
\newcommand{\CalA}{\mathcal{A}}
\newcommand{\CalC}{\mathcal{C}}
\newcommand{\CalF}{\mathcal{F}}
\newcommand{\CalG}{\mathcal{G}}
\newcommand{\CalP}{\mathcal{P}}
\newcommand{\CalM}{\mathcal{M}}
\newcommand{\CalN}{\mathcal{N}}
\newcommand{\CalR}{\mathcal{R}}
\newcommand{\CalS}{\mathcal{S}}
\newcommand{\CalX}{\mathcal{X}}

% \newcommand{\id}{\mathrm{id}}
\newcommand{\pad}{\mathrm{pad}}
% \newcommand{\dom}{\mathrm{dom}}
%\newcommand{\modulo}{\; \mathrm{mod}}
\newcommand{\range}{\mathrm{range}}
\newcommand{\pair}[1]{\langle #1 \rangle}

\newcommand{\unpair}{\mathrm{unpair}}

\newcommand{\eqnComment}[2]{\underset{{\scriptstyle \text{#1}}}{#2}}

\DeclareMathOperator{\modulo}{mod}
\DeclareMathOperator{\Pow}{Pow}
