# Supplementary material for: Theory of Stochastic Drift
Source: arXiv:2406.14589 source file (2024-06-19)
Supplement: Supplementary file 2 [file additional_packages.tex]

\usepackage{scrlayer-scrpage}
\usepackage{lastpage}

\usepackage{mdframed}
%\usepackage[theorems]{tcolorbox}

\usepackage[normalem]{ulem}

\usepackage{listings}
\lstset{%
    mathescape,
    frame=single
}

\renewcommand*{\footnoterule}{\rule{0 pt}{0 pt}}
\deffootnote[1.2 em]{1.2 em}{0 em}{\makebox[1.4 em][l]{\textbf{\thefootnotemark}}}

\newcommand{\assign}{\leftarrow}
